# Supplementary material for: On the Audio-visual Synchronization for Lip-to-Speech Synthesis
Source: arXiv:2303.00502 source file (2023-03-01)
Supplement: Supplementary file 1 [file appendix.tex]

\section{Appendix}

\begin{algorithm}
	\caption{PyTorch-like pseudocode for computing the synchronization vector.}
	\label{algo:asm}
	\begin{minted}
[
fontsize=\footnotesize,
baselinestretch=1.0
]
{python}
"""
Args:
    d_f: feature channels, d_m, mel channels
    t: length of upsampled video features and mel
    v: upsampled video features (d,t)
    m: video timewise 0/1 mask (1,t)
    a: audio mel-spectrogram (d_m,t)
    r: maximum synchronization radius
Return:
    s: synchronization vector
"""

# Extract local representation
v = v_conv(v) # (d,t)
a = a_conv(a) # (d,t)

# L2 normalization
v = normalize(v, dim=0)
a = normalize(a, dim=0)

# Pad and unfold along time, k=2r+1
v = F.pad(v, (r, r), dim=1) # (d,t+2r)
v = v.unfold(dim=1, size=t, step=1) # (d,k,t)
m = F.pad(m, (r, r), dim=1) # (1,t+2r)
m = m.unfold(dim=1, size=t, step=1) # (1,k,t)

# Repeat the audio feature
a = a.unsqueeze(1) #(d,1,t)
a = a.repeat_interleave(k, dim=1) # (d,k,t)

# Compute synchronization vector
s = einsum("dkt,dt->k", v * m, a * m)
s = s / m.sum(dim=[0,2])

return s

\end{minted}
\end{algorithm}
